# Supplementary material for: Selected Machine Learning of HOMO-LUMO gaps with Improved Data-Efficiency
Source: arXiv:2110.02596 source file (2021-10-06)
Supplement: Supplementary file 2 [file si_preamble.tex]

\usepackage{amsthm}
\usepackage{mathtools}
\usepackage{physics}
\usepackage{xcolor}
\usepackage{graphicx}
\usepackage[left=23mm,right=13mm,top=35mm,columnsep=15pt]{geometry} 
\usepackage{adjustbox}
\usepackage{placeins}
\usepackage[T1]{fontenc}
\usepackage{lipsum}
\usepackage{csquotes}
